# Supplementary material for: First-principles thermodynamics of CsSnI3
Source: arXiv:2301.10071 source file (2023-01-24)
Supplement: Supplementary file 1 [file convergence.tex]

\section{DFT convergence tests}

In this section we investigate the convergence with the DFT parameters.
Calculations are performed on the cubic structure with 20 atoms per unit cell.

The pseudopotentials employed are norm conserving (NC) from Pseudo-Dojo library (accuracy standard) computed with the PBEsol functional.

In \figurename~\ref{fig:cutoff:conv} we report the convergence of the energy, forces and stress tensor with the DFT cutoff.

\begin{figure}[hbtp]
	\centering
	\includegraphics[width=\textwidth]{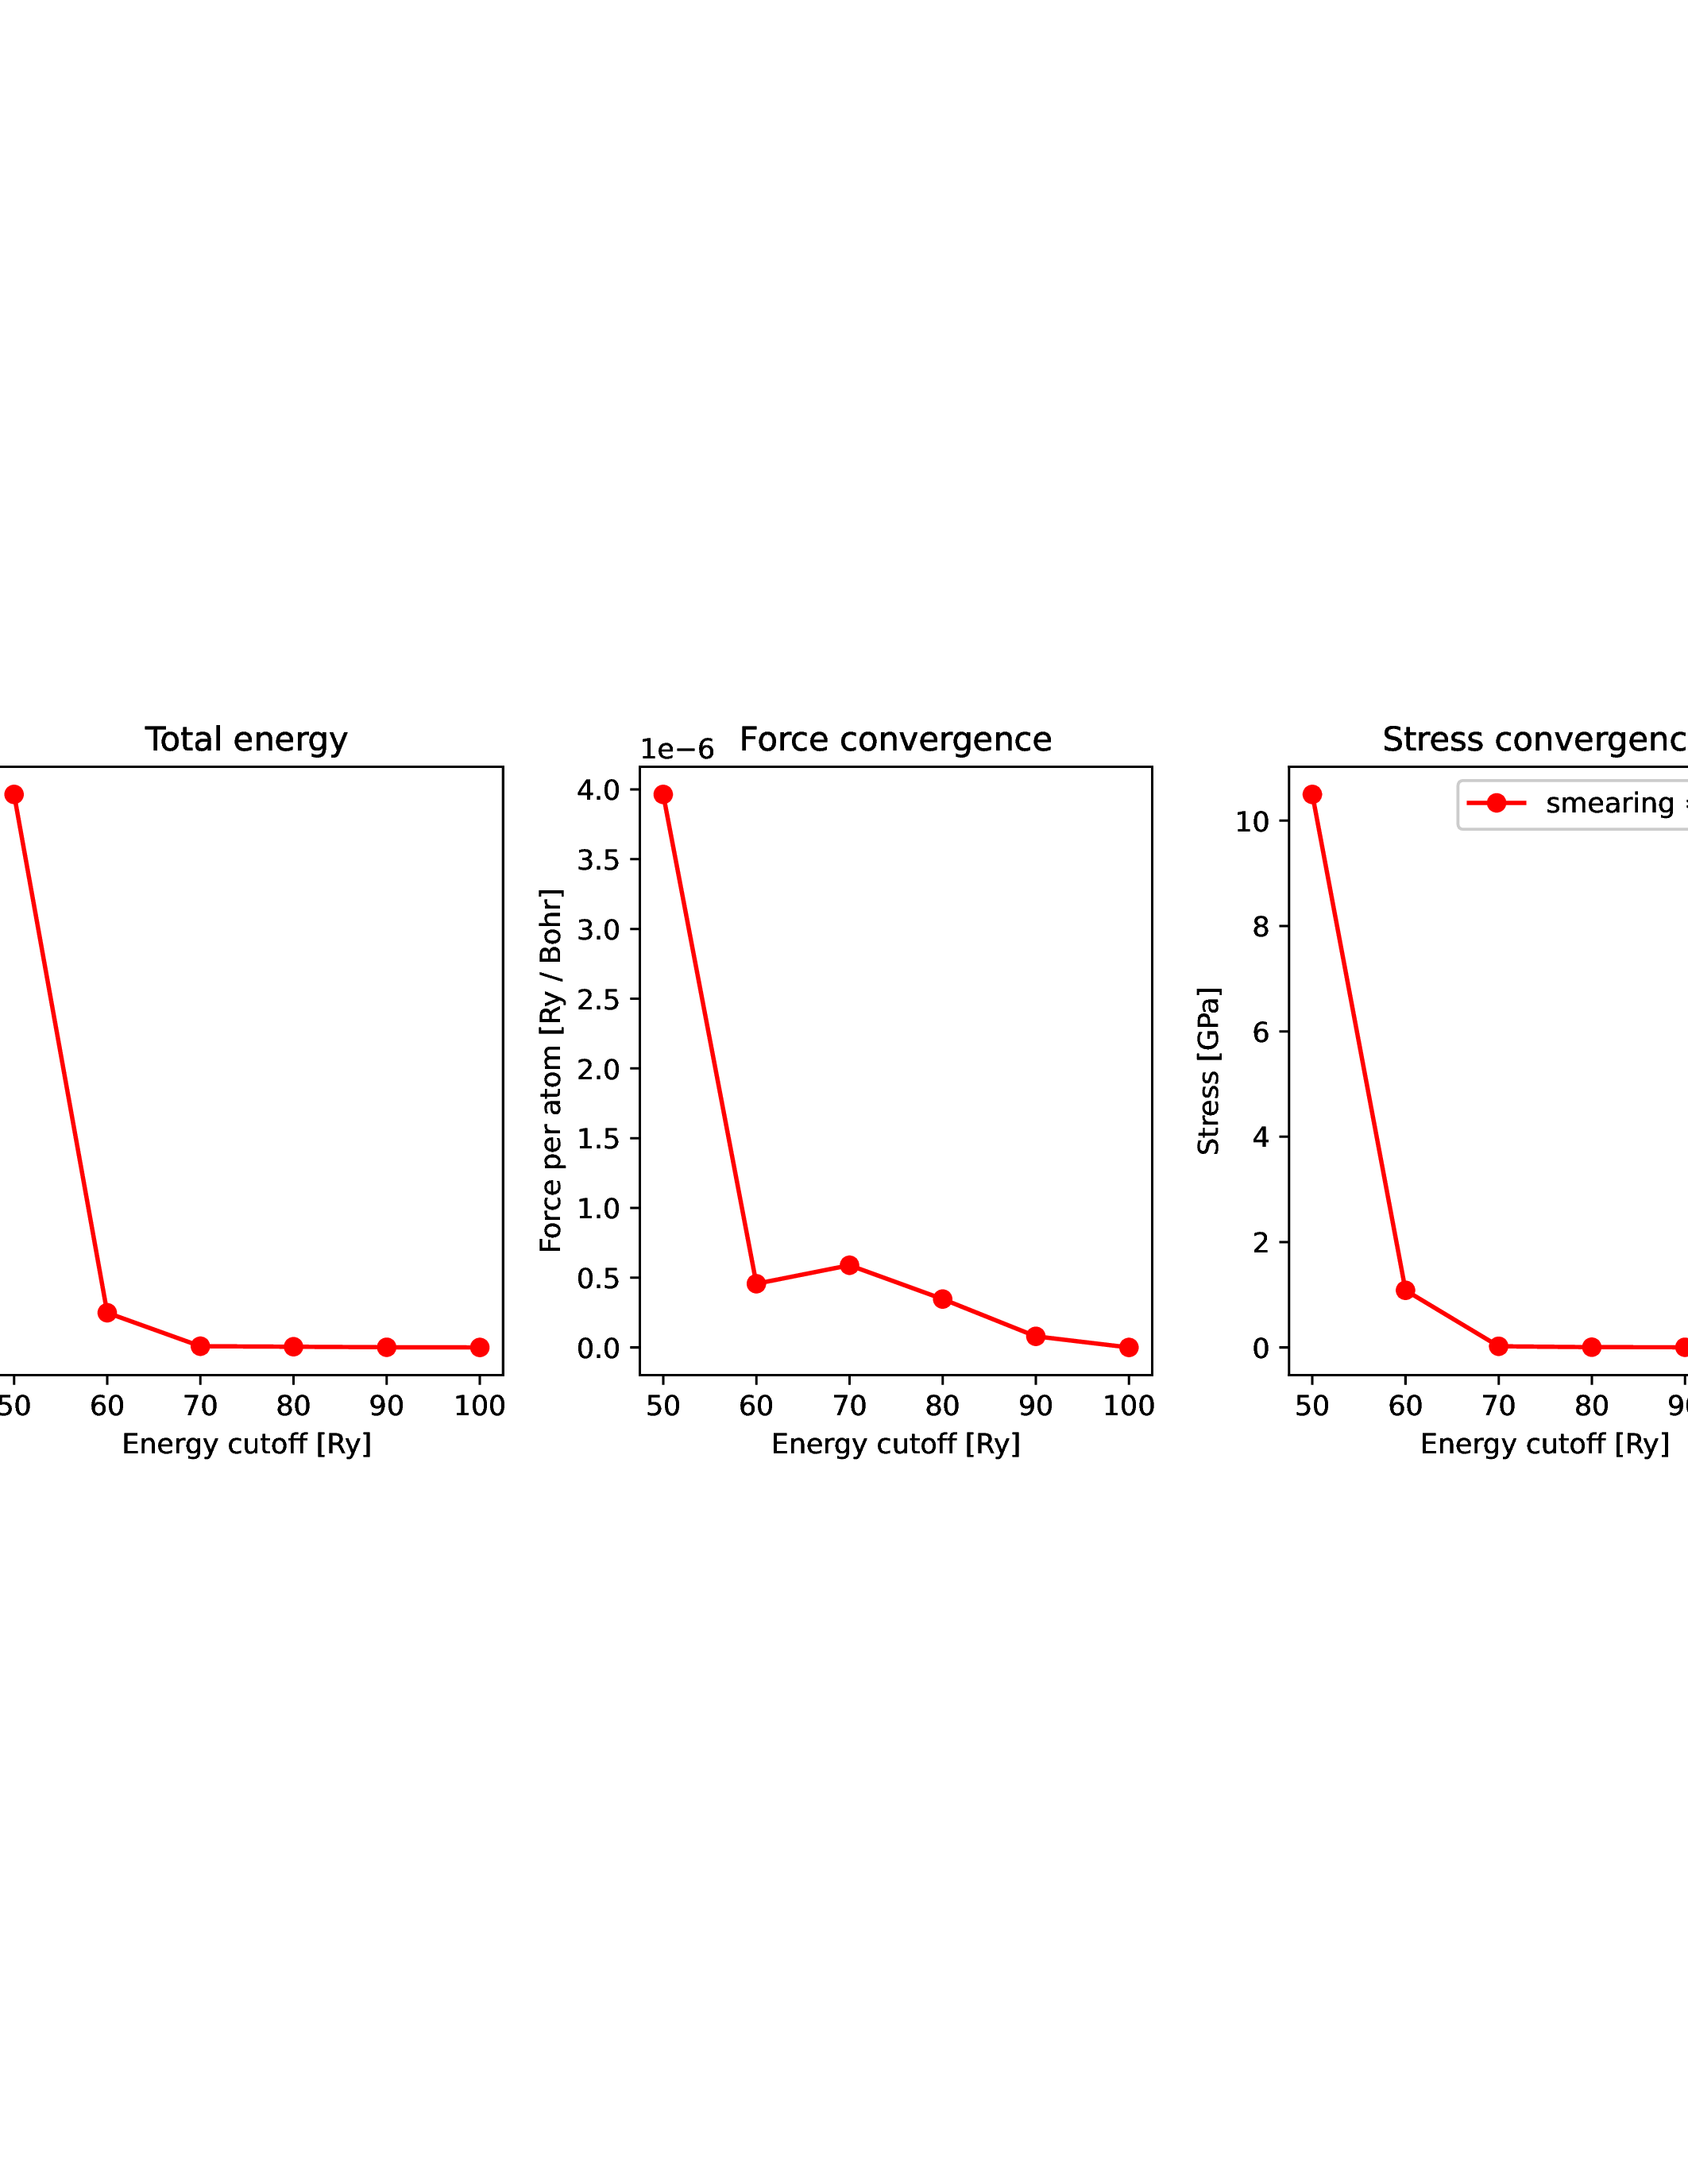}
	\caption{Convergence with the wavefunction cutoff of the total energy, force and stress tensor. The structure on which the cutoff is computed contain 20 atoms per unit cell with 8 symmetries, K points 4x4x4 with a 1 1 1 offset. The self-concistency is stopped with a threshold of \SI{1e-10}{\rydberg}.
	}
	\label{fig:cutoff:conv}
\end{figure}

As clearly reported, with a cutoff on the wavefunction of \SI{70}{\rydberg} the calculation is at convergence for both force, energy and stress tensor.

The convergence with the number of k-points has been computed with the PBE functional and PAW pseudopotential from PSL version 1.0.0, a cutoff of \SI{47}{\rydberg} for the wavefunction and \SI{376}{\rydberg} for the electron density. Th results are reported in \figurename~\ref{fig:kpts:conv}

\begin{figure}[hbtp]
	\centering
	\includegraphics[width=\textwidth]{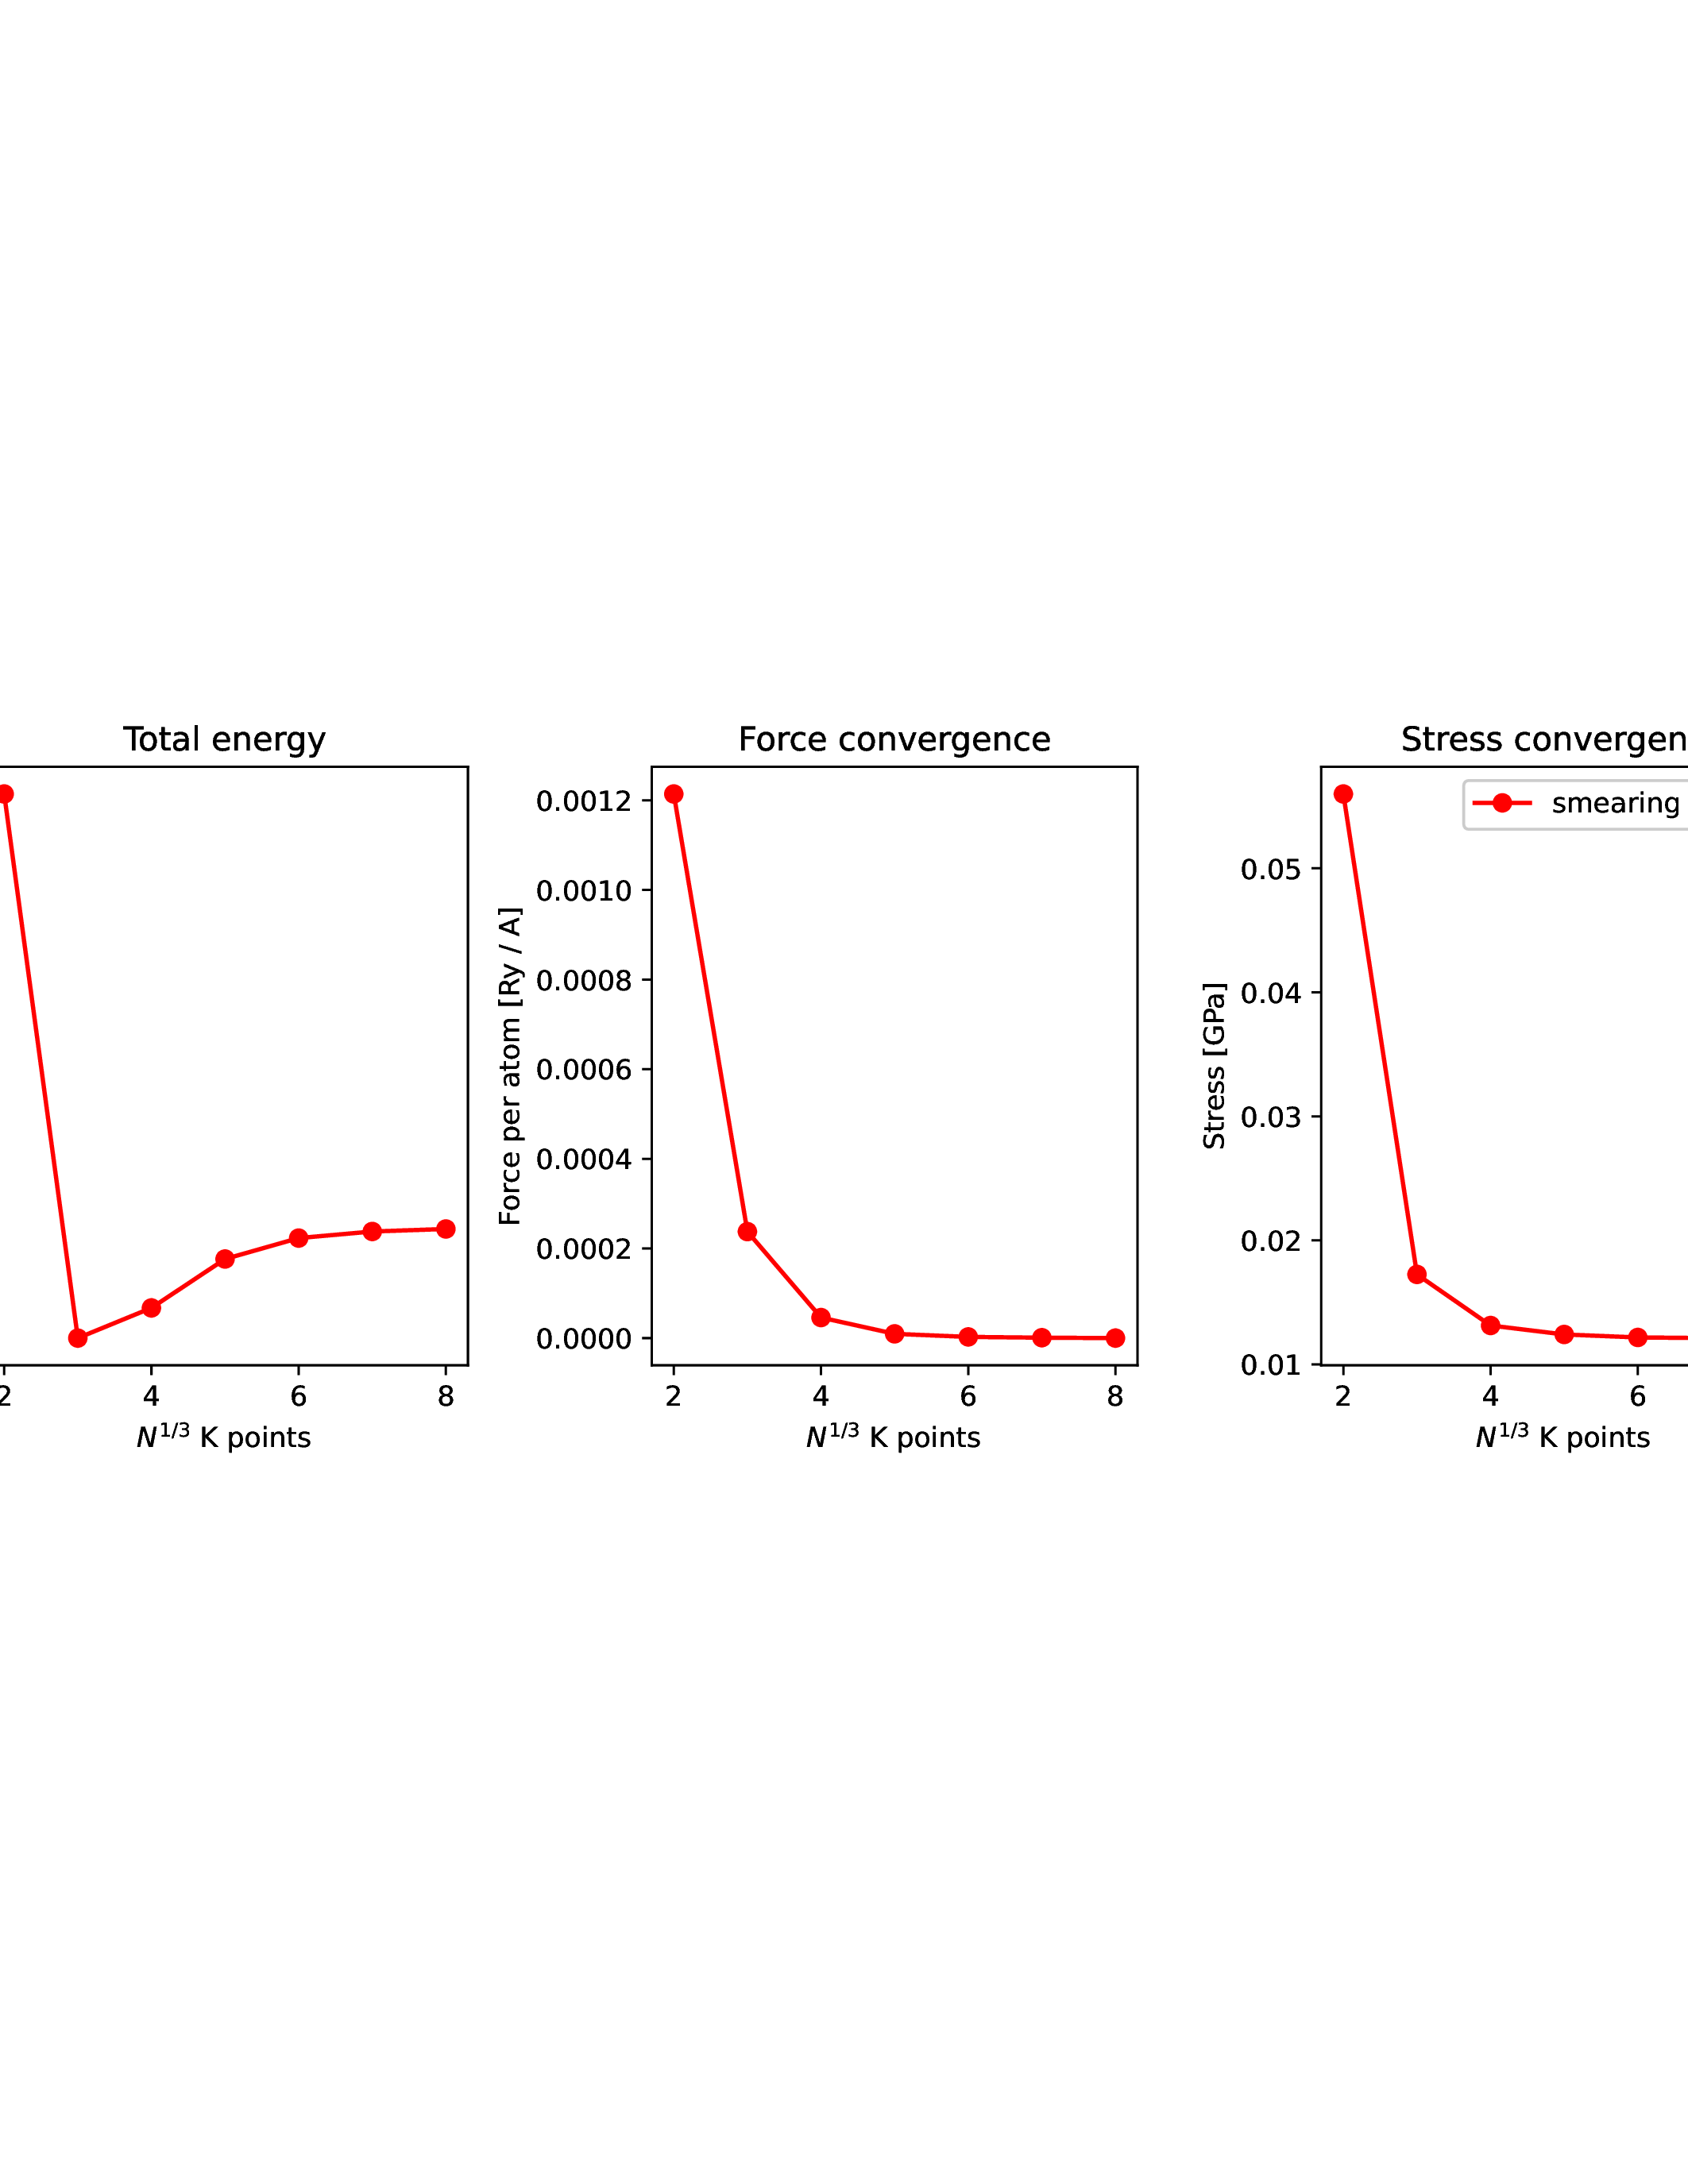}
	\caption{Convergencen of the k point mesh. The mesh is a NxNxN grid with offset of 1 1 1.\label{fig:kpts:conv}}
\end{figure}

Satisfactory results are already achieved with a 4x4x4 k-mesh and can be extended in a 6x6x6 for highly converged results.

\subsection{Fourier interpolation}

To assess which is the error of the interpolation, we computed the harmonic dynamical matrix for the cubic phase in a 2x2x2, 3x3x3 and 4x4x4 centered q-mesh and performed the Fourier interpolation on the $\Gamma-M-R-\Gamma-X$ q-path.

We report the results in \figurename~\ref{fig:fourier:conv:harm}.

\textbf{TODO: add effective charges to wash out nonanalytic terms.}

\begin{figure}[hbtp]
	\centering
	\includegraphics[width=0.8\textwidth]{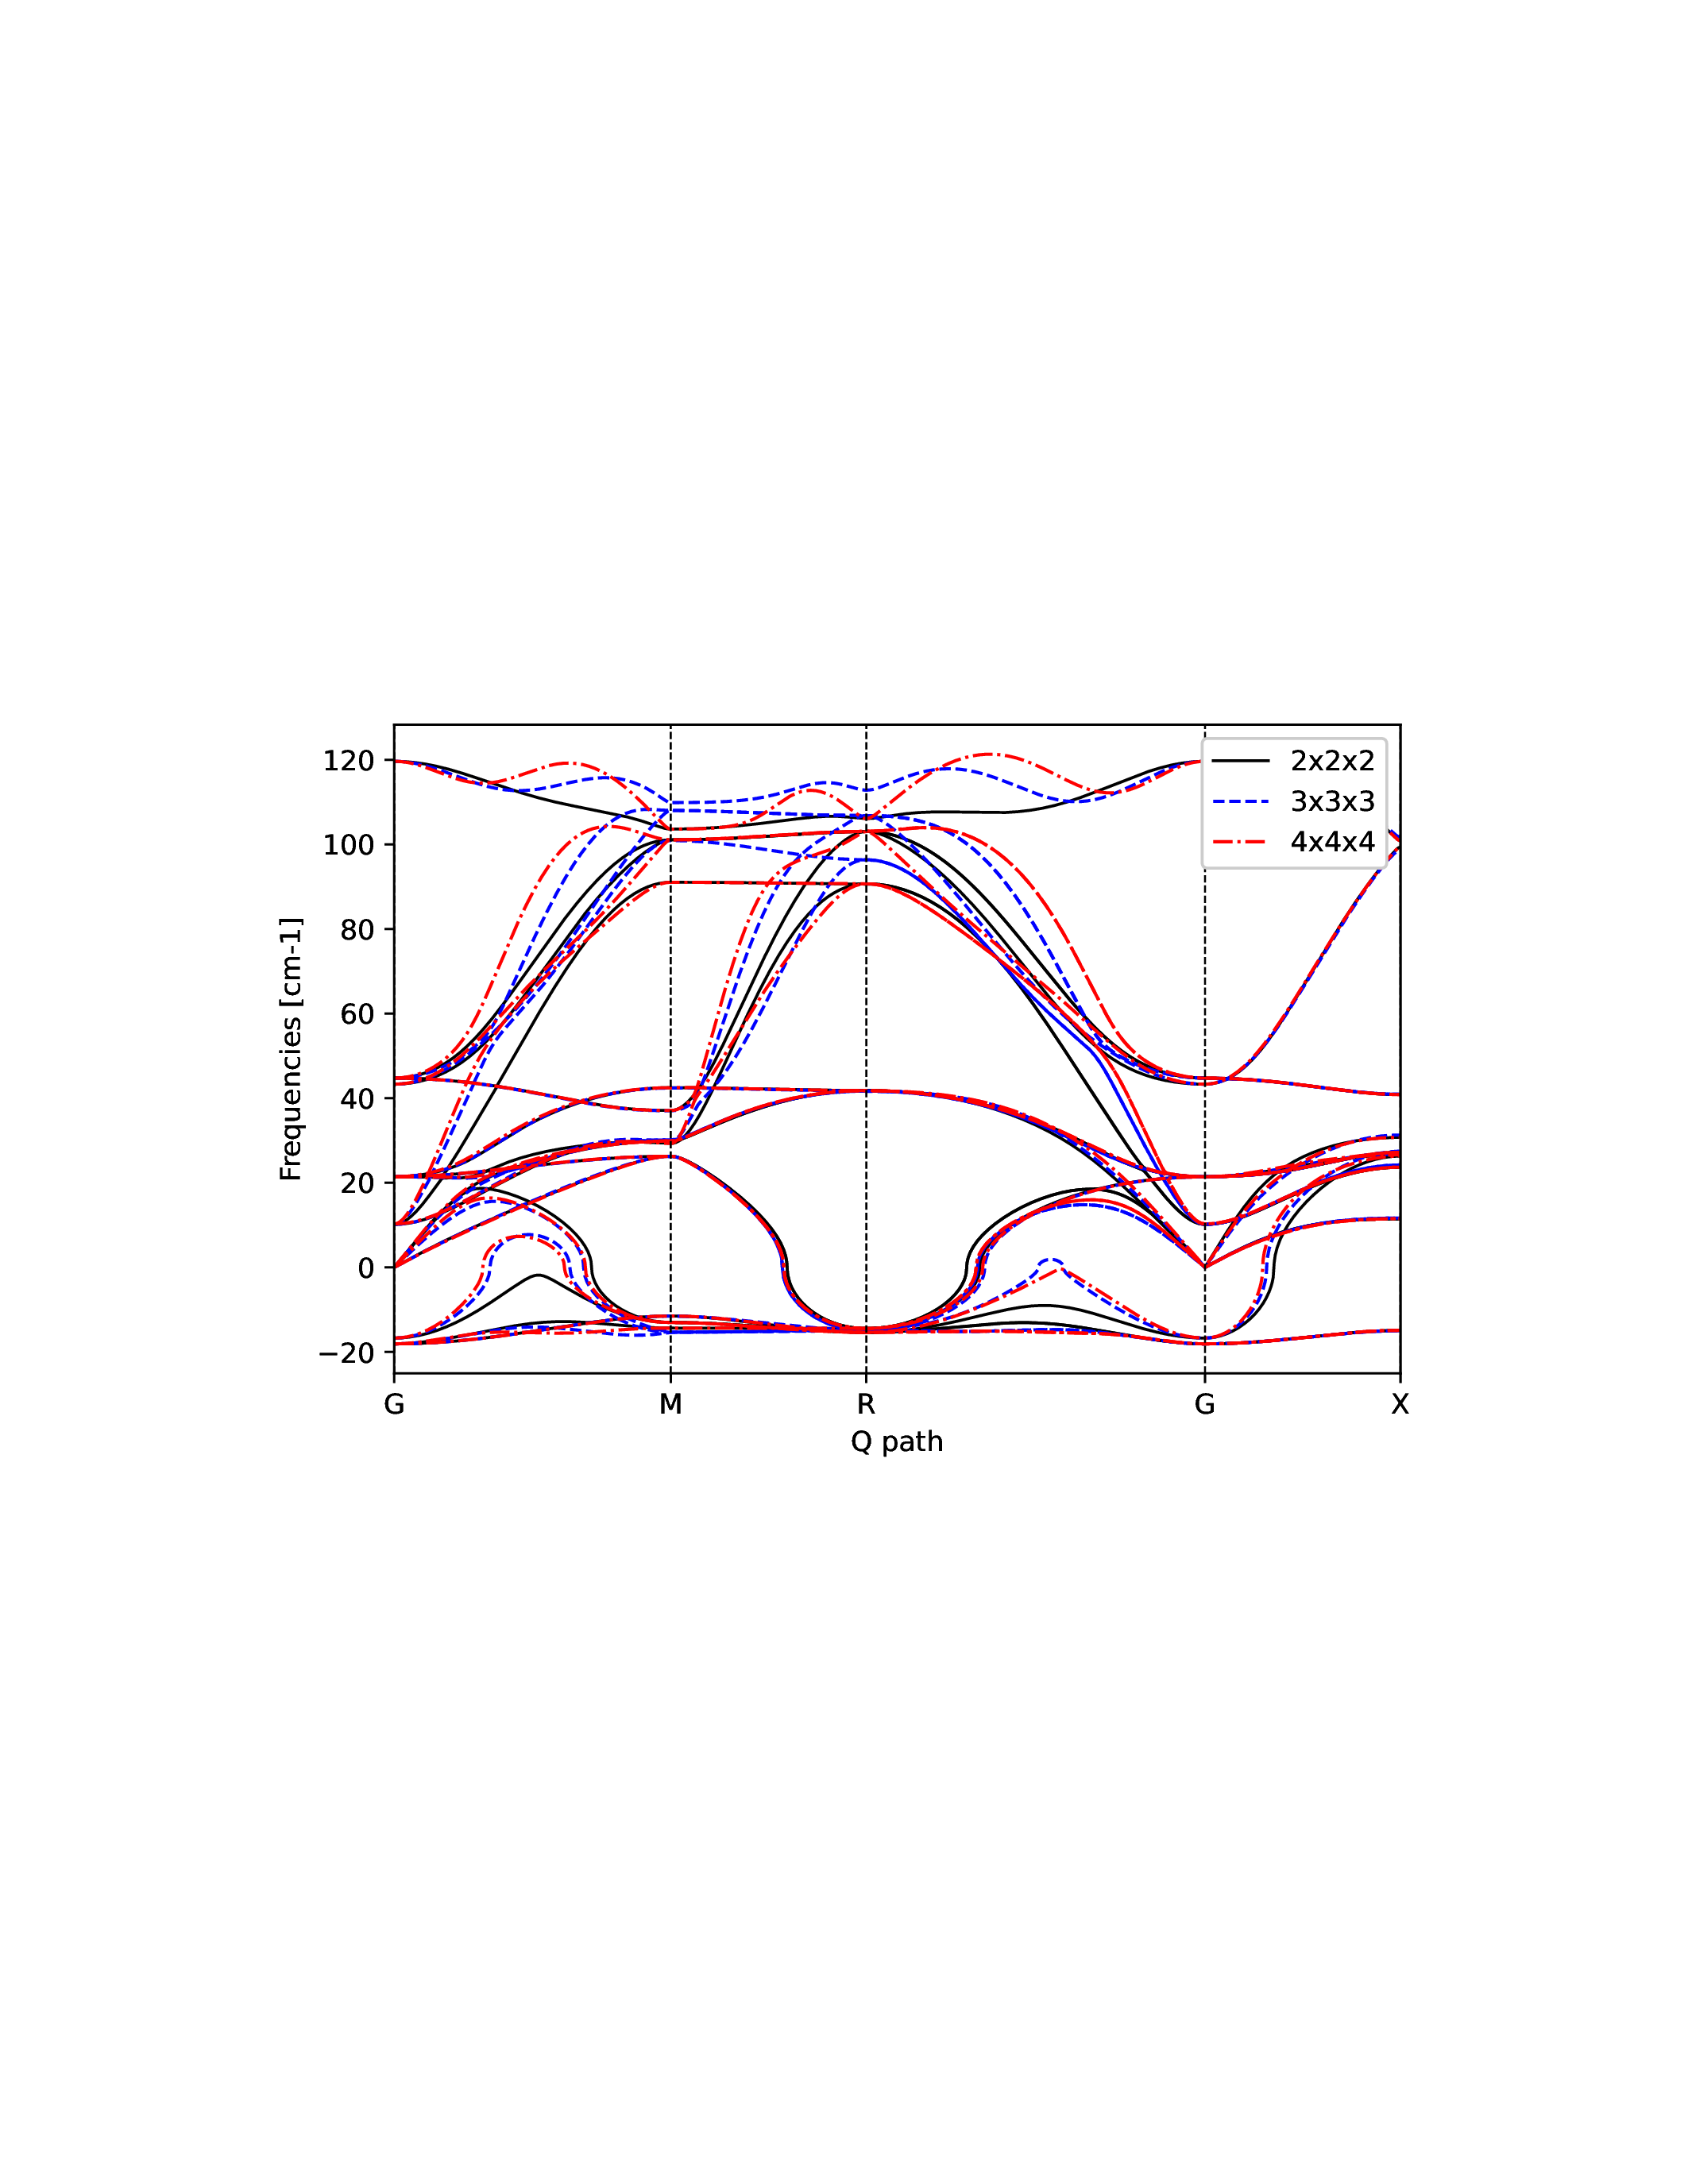}
	\caption{Convergence of the phonon dispersion interpolated with Fourier interpolation.}
	\label{fig:fourier:conv:harm}
\end{figure}

The instability along the path of the optical mode is well described by a 3x3x3 already: the 2x2x2 supercell correctly grasp the $M$ and $R$ (which are the q-points of the instability), but fails in grasping the $\Gamma-R$ and $\Gamma-R$ dispersion. In the 3x3x3 both the $M$ and $R$ points are interpolated, but their frequency correctly matches the frequency. The things are different for the highest optical modes, but they could be affected by the nonanaliticity of the effective charges which are not included here.
