# Supplementary material for: First-principles thermodynamics of CsSnI3
Source: arXiv:2301.10071 source file (2023-01-24)
Supplement: Supplementary file 2 [file results_222.tex]

\section{Convergence}

We performed the calculation of the SSCHA in the 2x2x2 supercell (40 atoms).

We report the hessian at $T = \SI{300}{\kelvin}$ and $\SI{800}{\kelvin}$.

Experimentally the transition temperature in the cubic phase is around $\SI{500}{\kelvin}$.

We report in \figurename~\ref{fig:sscha:dyn} the dispersion of the SCHA auxiliary phonons at these two temperatures.

\begin{figure}[hbtp]
	\centering
	\includegraphics[width=0.8\textwidth]{scha.eps}
	\caption{Auxiliary frequencies of the SSCHA dispersion as a function of temperature.}
	\label{fig:sscha:dyn}
\end{figure}

Phonons became stiffer as we increase the temperature. The temperature dependence of the SSCHA phonons is quite remarkable and involves all optical and acoustic branches. This underlines a dominant role of anharmonicity in the thermodynamics of the cubic perovskites.

We can study the structural stability. This is done computing the free energy hessian of the structure.
This calculation can be done at two levels: the full hessian, which require the inversion of a matrix of $N^2\times N^2$, with $N$ the number of atoms in the supercell, or the bubble approximation.

The full hessian calculation is affordable in supercells up to the 2x2x2. Already in the 3x3x3, only to store the fourth order force constant tensor requires \SI{200}{\giga\byte} of RAM. 

In \figurename~\ref{fig:bubble:T} we report the result of the Hessian calculation computed with the bubble approximation. This approximation worked very well in almost all materials studied up to now with the SCHA.

\begin{figure}
	\centering
	\includegraphics[width=0.8\textwidth]{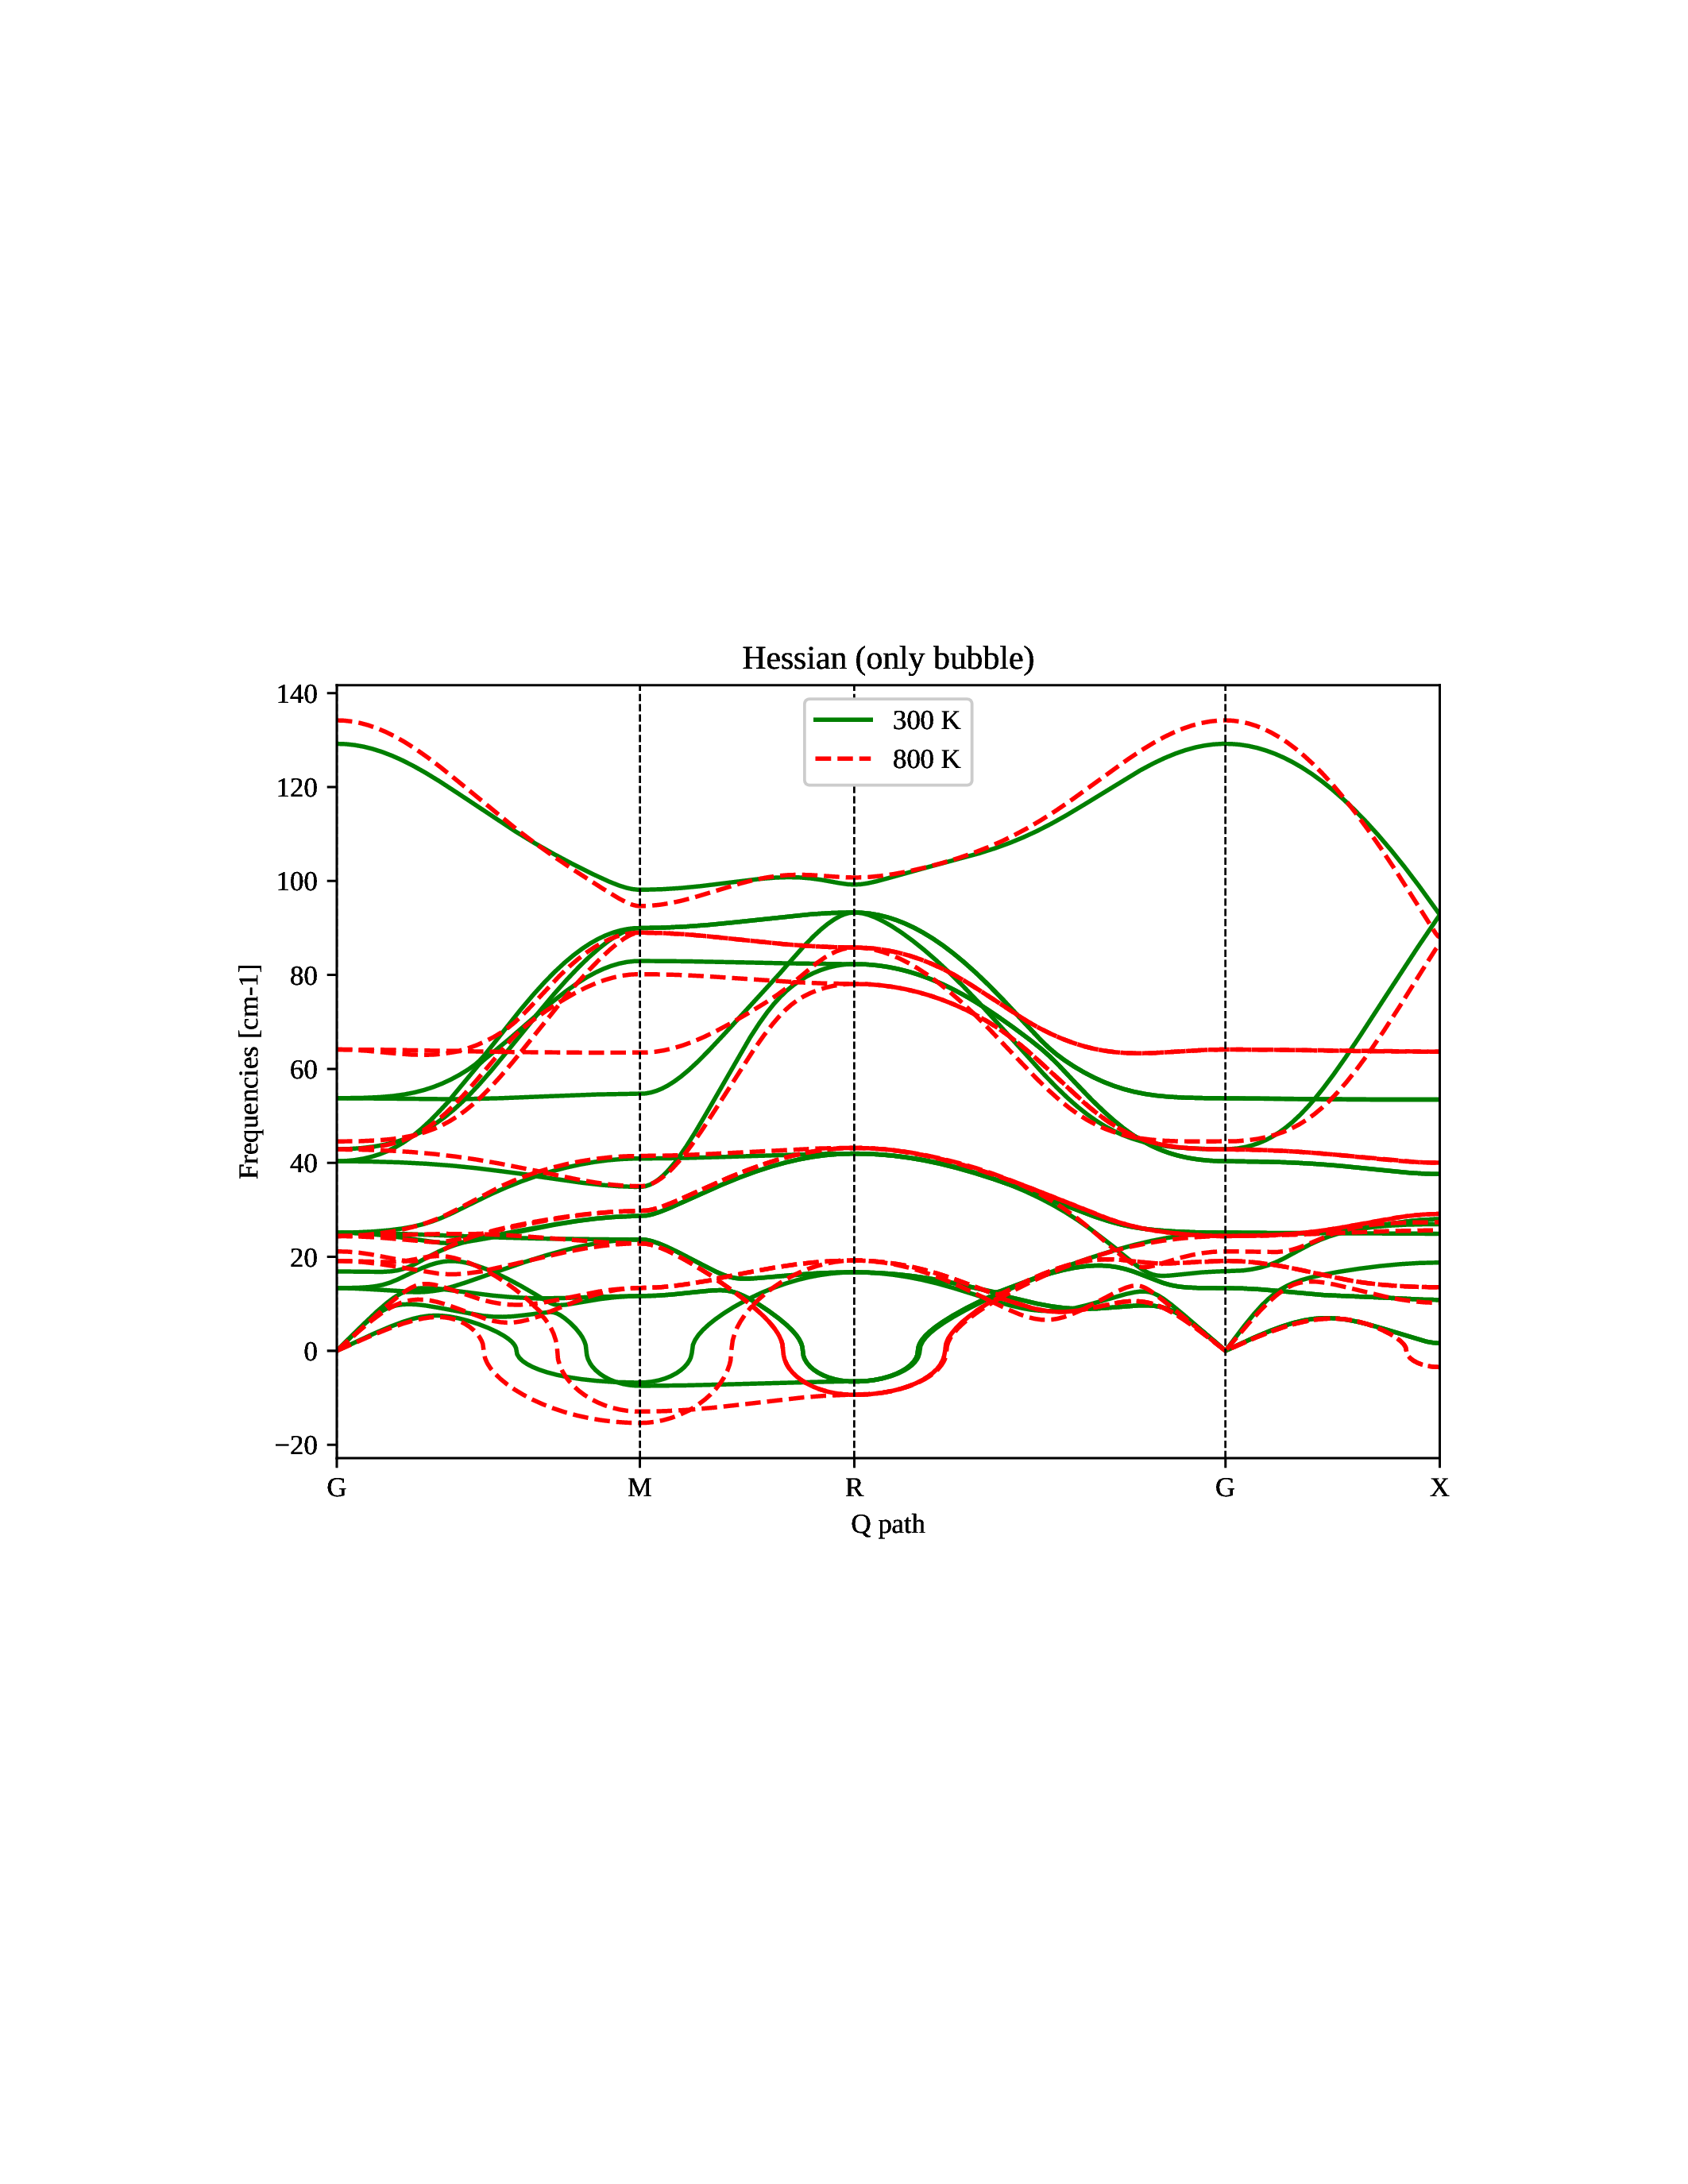}
	\caption{Free energy hessian versus temperature in the bubble approximation, computed in a 2x2x2 supercell and Fourier interpolated.\label{fig:bubble:T}}
\end{figure}

From the bubble approximation of the Hessian we see that the cubic structure is unstable at all temperature (even at \SI{800}{\kelvin}), in stark disagreement with experiments, which shows the cubic phase to become stable after $\SI{500}{\kelvin}$. Moreover, the imaginary phonons seem to become even more imaginary at higher temperatures, which is odd.

To check if this is the bubble approximation, we repeated also the calculation with the full hessian method, which is possible only up to the 2x2x2 supercell.
The results are shown in \figurename~\ref{fig:hessian:T}.

\begin{figure}
	\centering
	\includegraphics[width=0.8\textwidth]{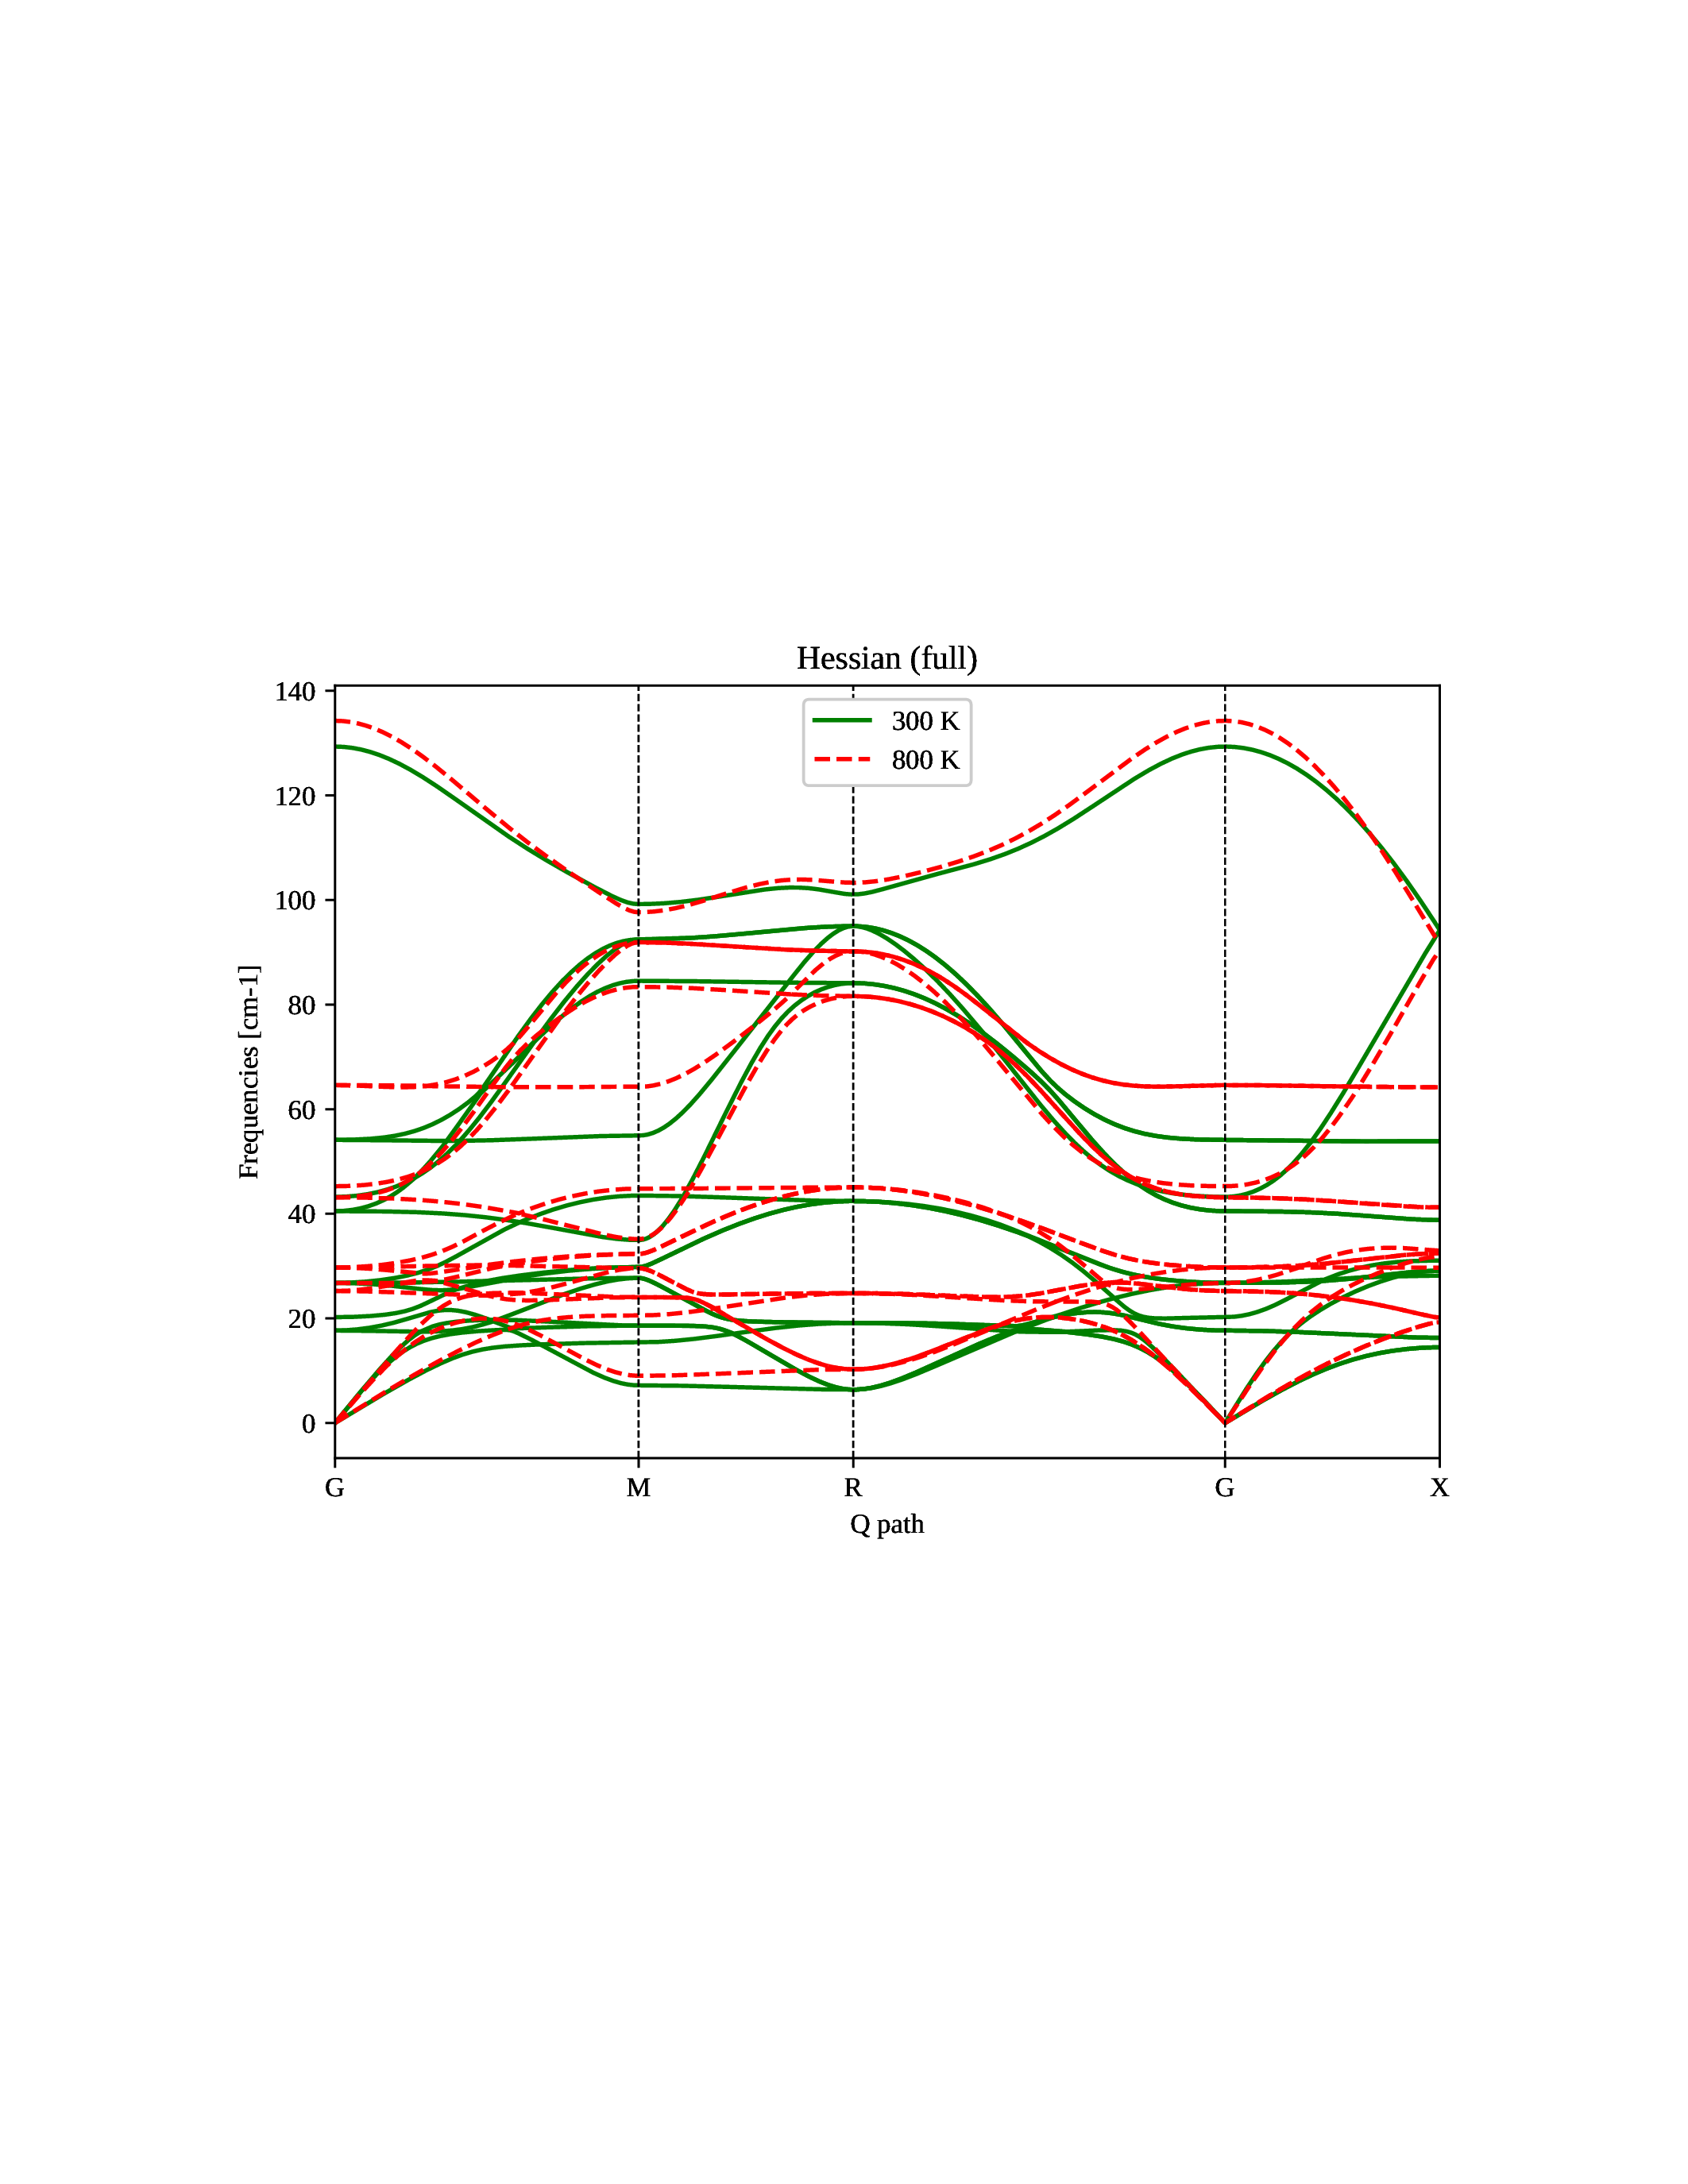}
	\caption{Free energy hessian versus temperature without approximation (SCHA), computed in the 2x2x2 supercell and Fourier interpolated.\label{fig:hessian:T}}
\end{figure}

The results are in contrast with the bubble approximation, making \ch{CsSnI3} the first system under analysis which requires the calculation of the full bubble to study the stability. Here, we see that the cubic structure is stable already at \SI{300}{\kelvin}.

Stability of a structure means that this structure is a local minimum of the free energy, but does not assure that it is the global minimum and the ground state of the phase-diagram.

To further underline the difference, we report in \figurename~\ref{fig:v4:v3} the comparison between the full and the bubble approximation at \SI{300}{\kelvin}

\begin{figure}[hbtp]
	\centering
	\includegraphics[width=0.8\textwidth]{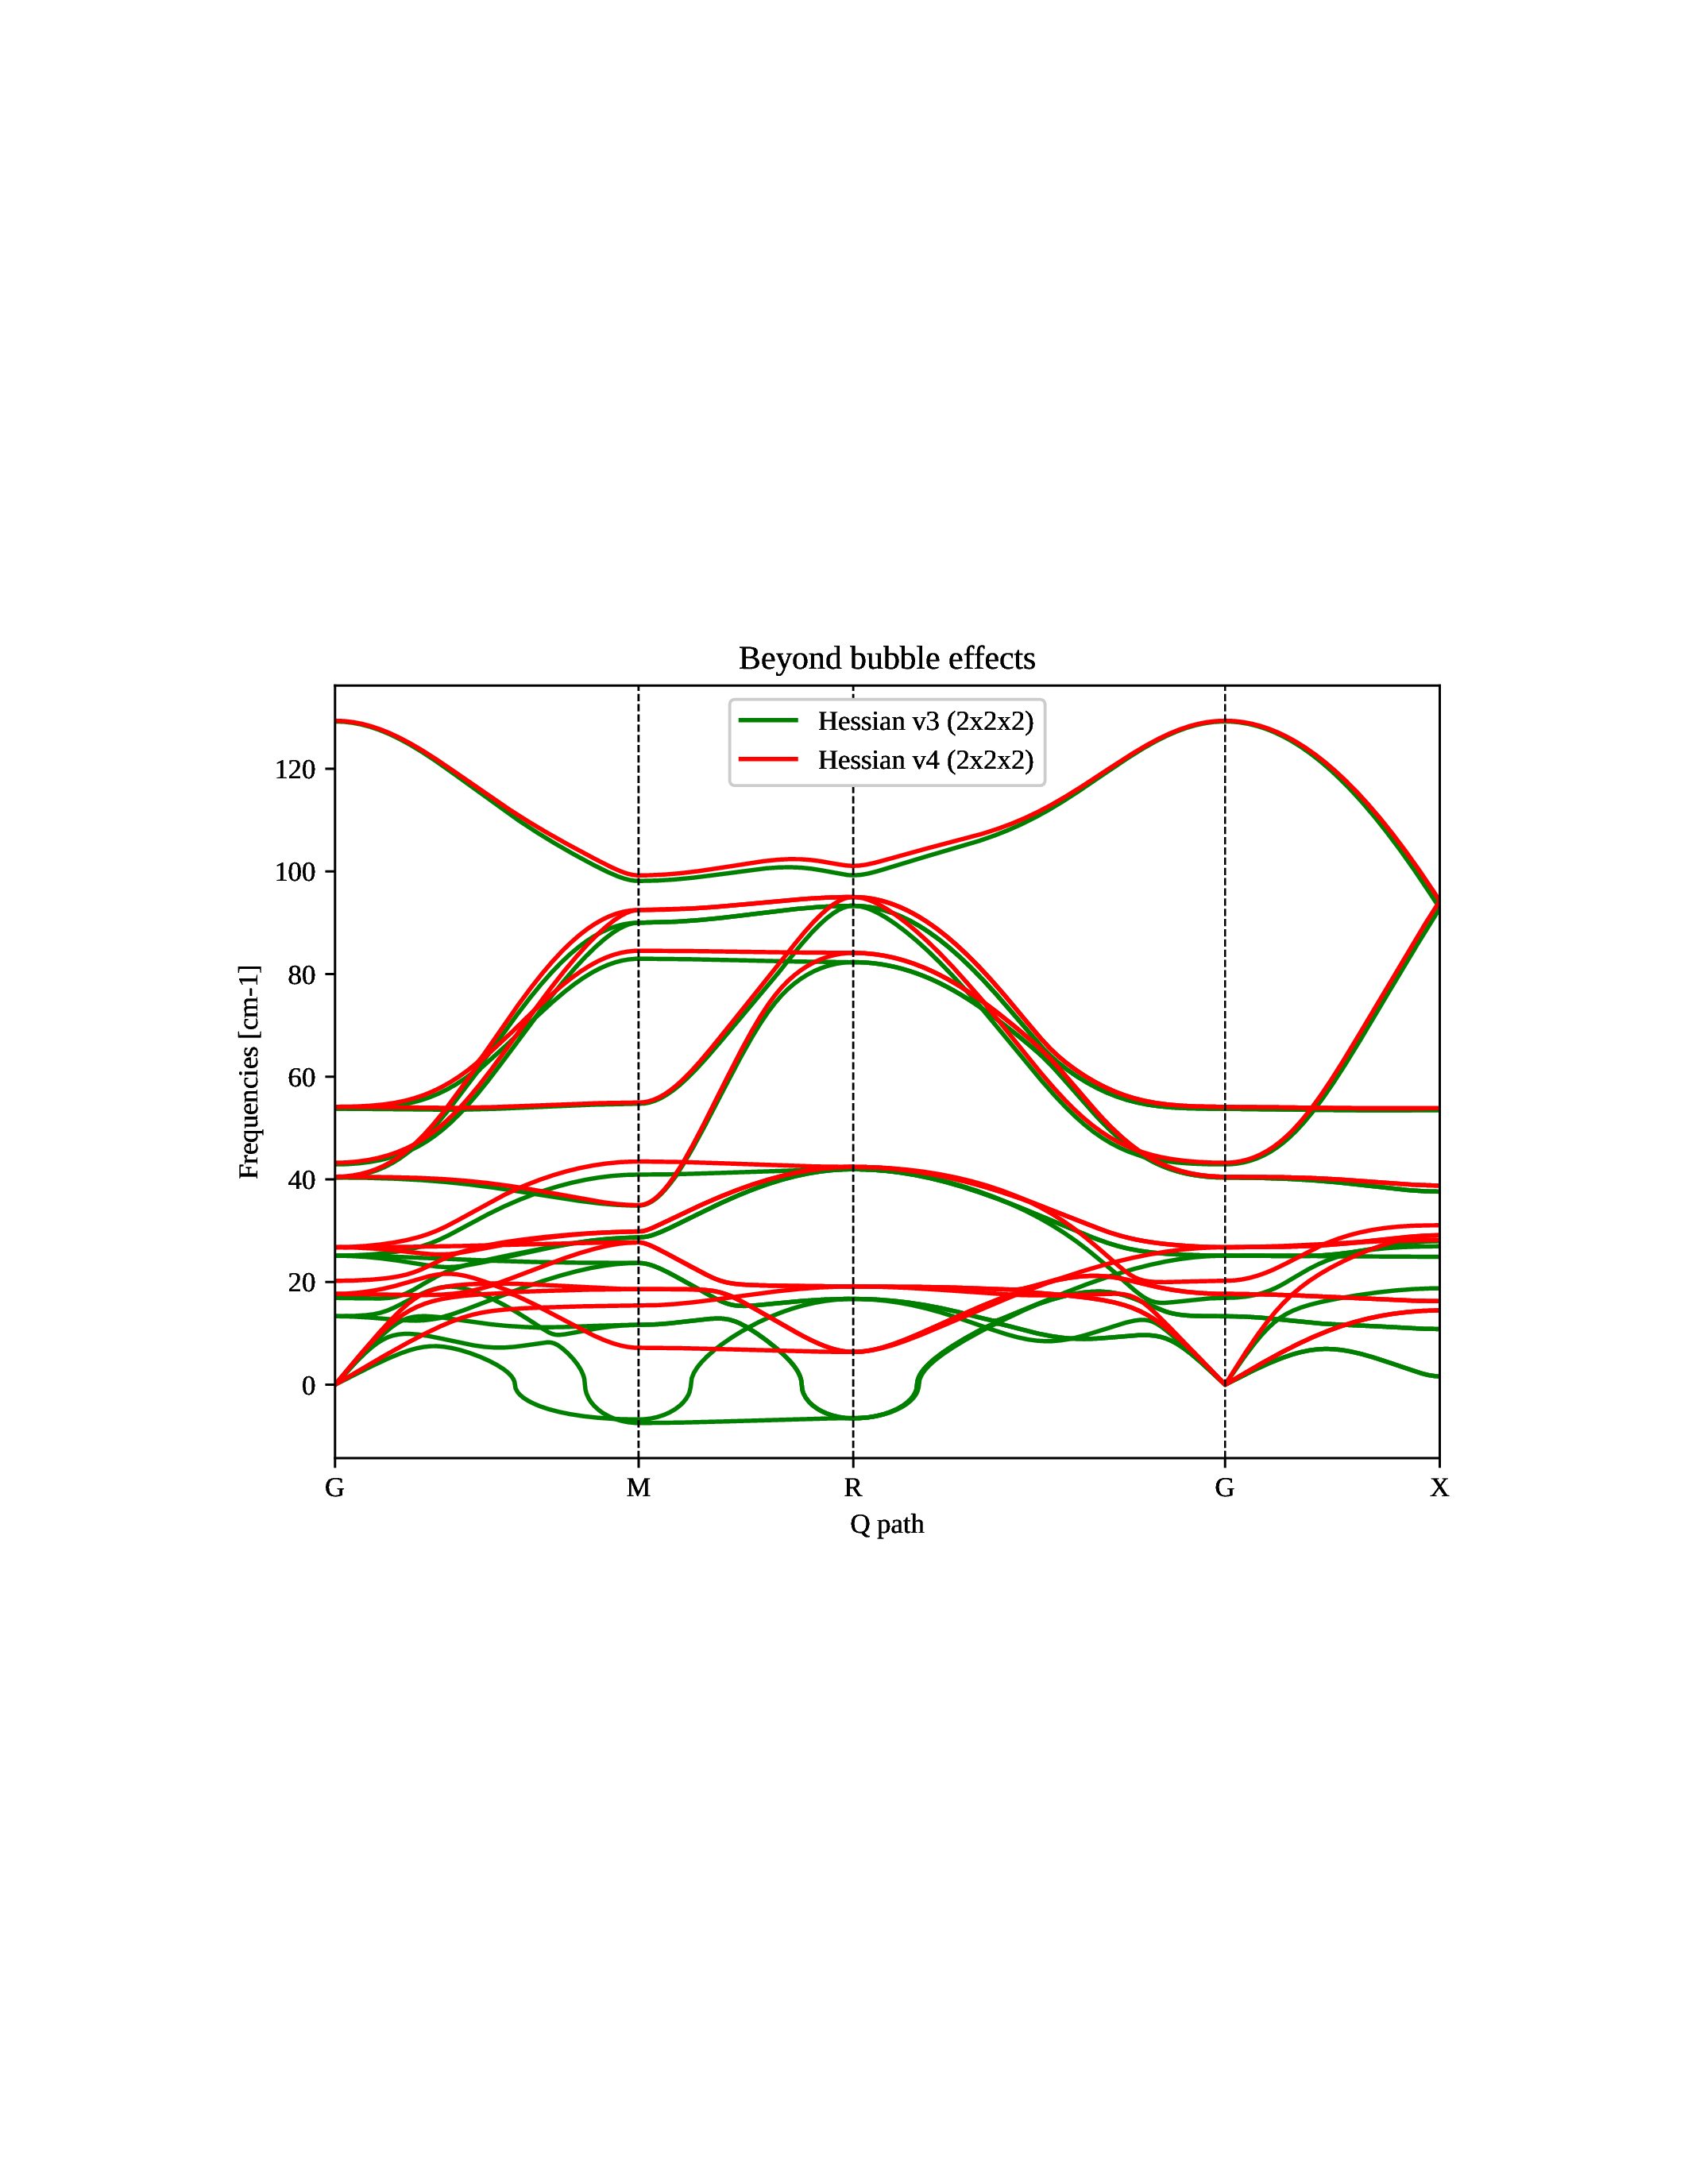}
	\caption{Comparison between the hessian in the bubble approximation (v3) and the full calculation (v4) at \SI{300}{\kelvin} in the 2x2x2 supercell.\label{fig:v4:v3}}
\end{figure}

For this reason we need to simulate also the other distortion and analyze the hypotesis of a first order phase-transition toward the cubic phase at \SI{500}{\kelvin} observed experimentally.
However, the stability of the \SI{300}{\kelvin} cubic phase of \ch{CsSnI3} could be an artifact of the small cell (2x2x2, 40 atoms) employed in the calculation. For this reasons, we repeated the SSCHA calculation up to the bubble approximation also in a bigger cell (3x3x3, 135 atoms).
Unfortunatley, in this cell we are not able to perform full hessian calculation.
