# Supplementary material for: First-principles thermodynamics of CsSnI3
Source: arXiv:2301.10071 source file (2023-01-24)
Supplement: Supplementary file 3 [file results_333.tex]

\subsection{3x3x3 convergence}

We computed the SSCHA also at $T = \SI{300}{\kelvin}$ in a bigger supercell, the 3x3x3 with 135 atoms, to assess the quality of the results obtained with the 4x4x4.

We report the convergence of the SSCHA phonons in \figurename~\ref{fig:sscha:conv}.

\begin{figure}
	\centering
	\includegraphics[width=0.8\textwidth]{scha_conv.eps}
	\caption{Convergence of the SSCHA auxiliary phonons in the 2x2x2 and the 3x3x3 supercell at \SI{300}{\kelvin}.\label{fig:sscha:conv}.}
\end{figure}

As can be seen, aside from the Fourier interpolation, which explains the differences of the high optical modes (see \figurename~\ref{fig:fourier:conv:harm}), the SSCHA result is already well converged in the 2x2x2 supercell.

We can also address the convergence of the Hessian calculation in the bubble approximation. The result is reported in \figurename~\ref{fig:bubble:conv}.

\begin{figure}
	\centering
	\includegraphics[width=0.8\textwidth]{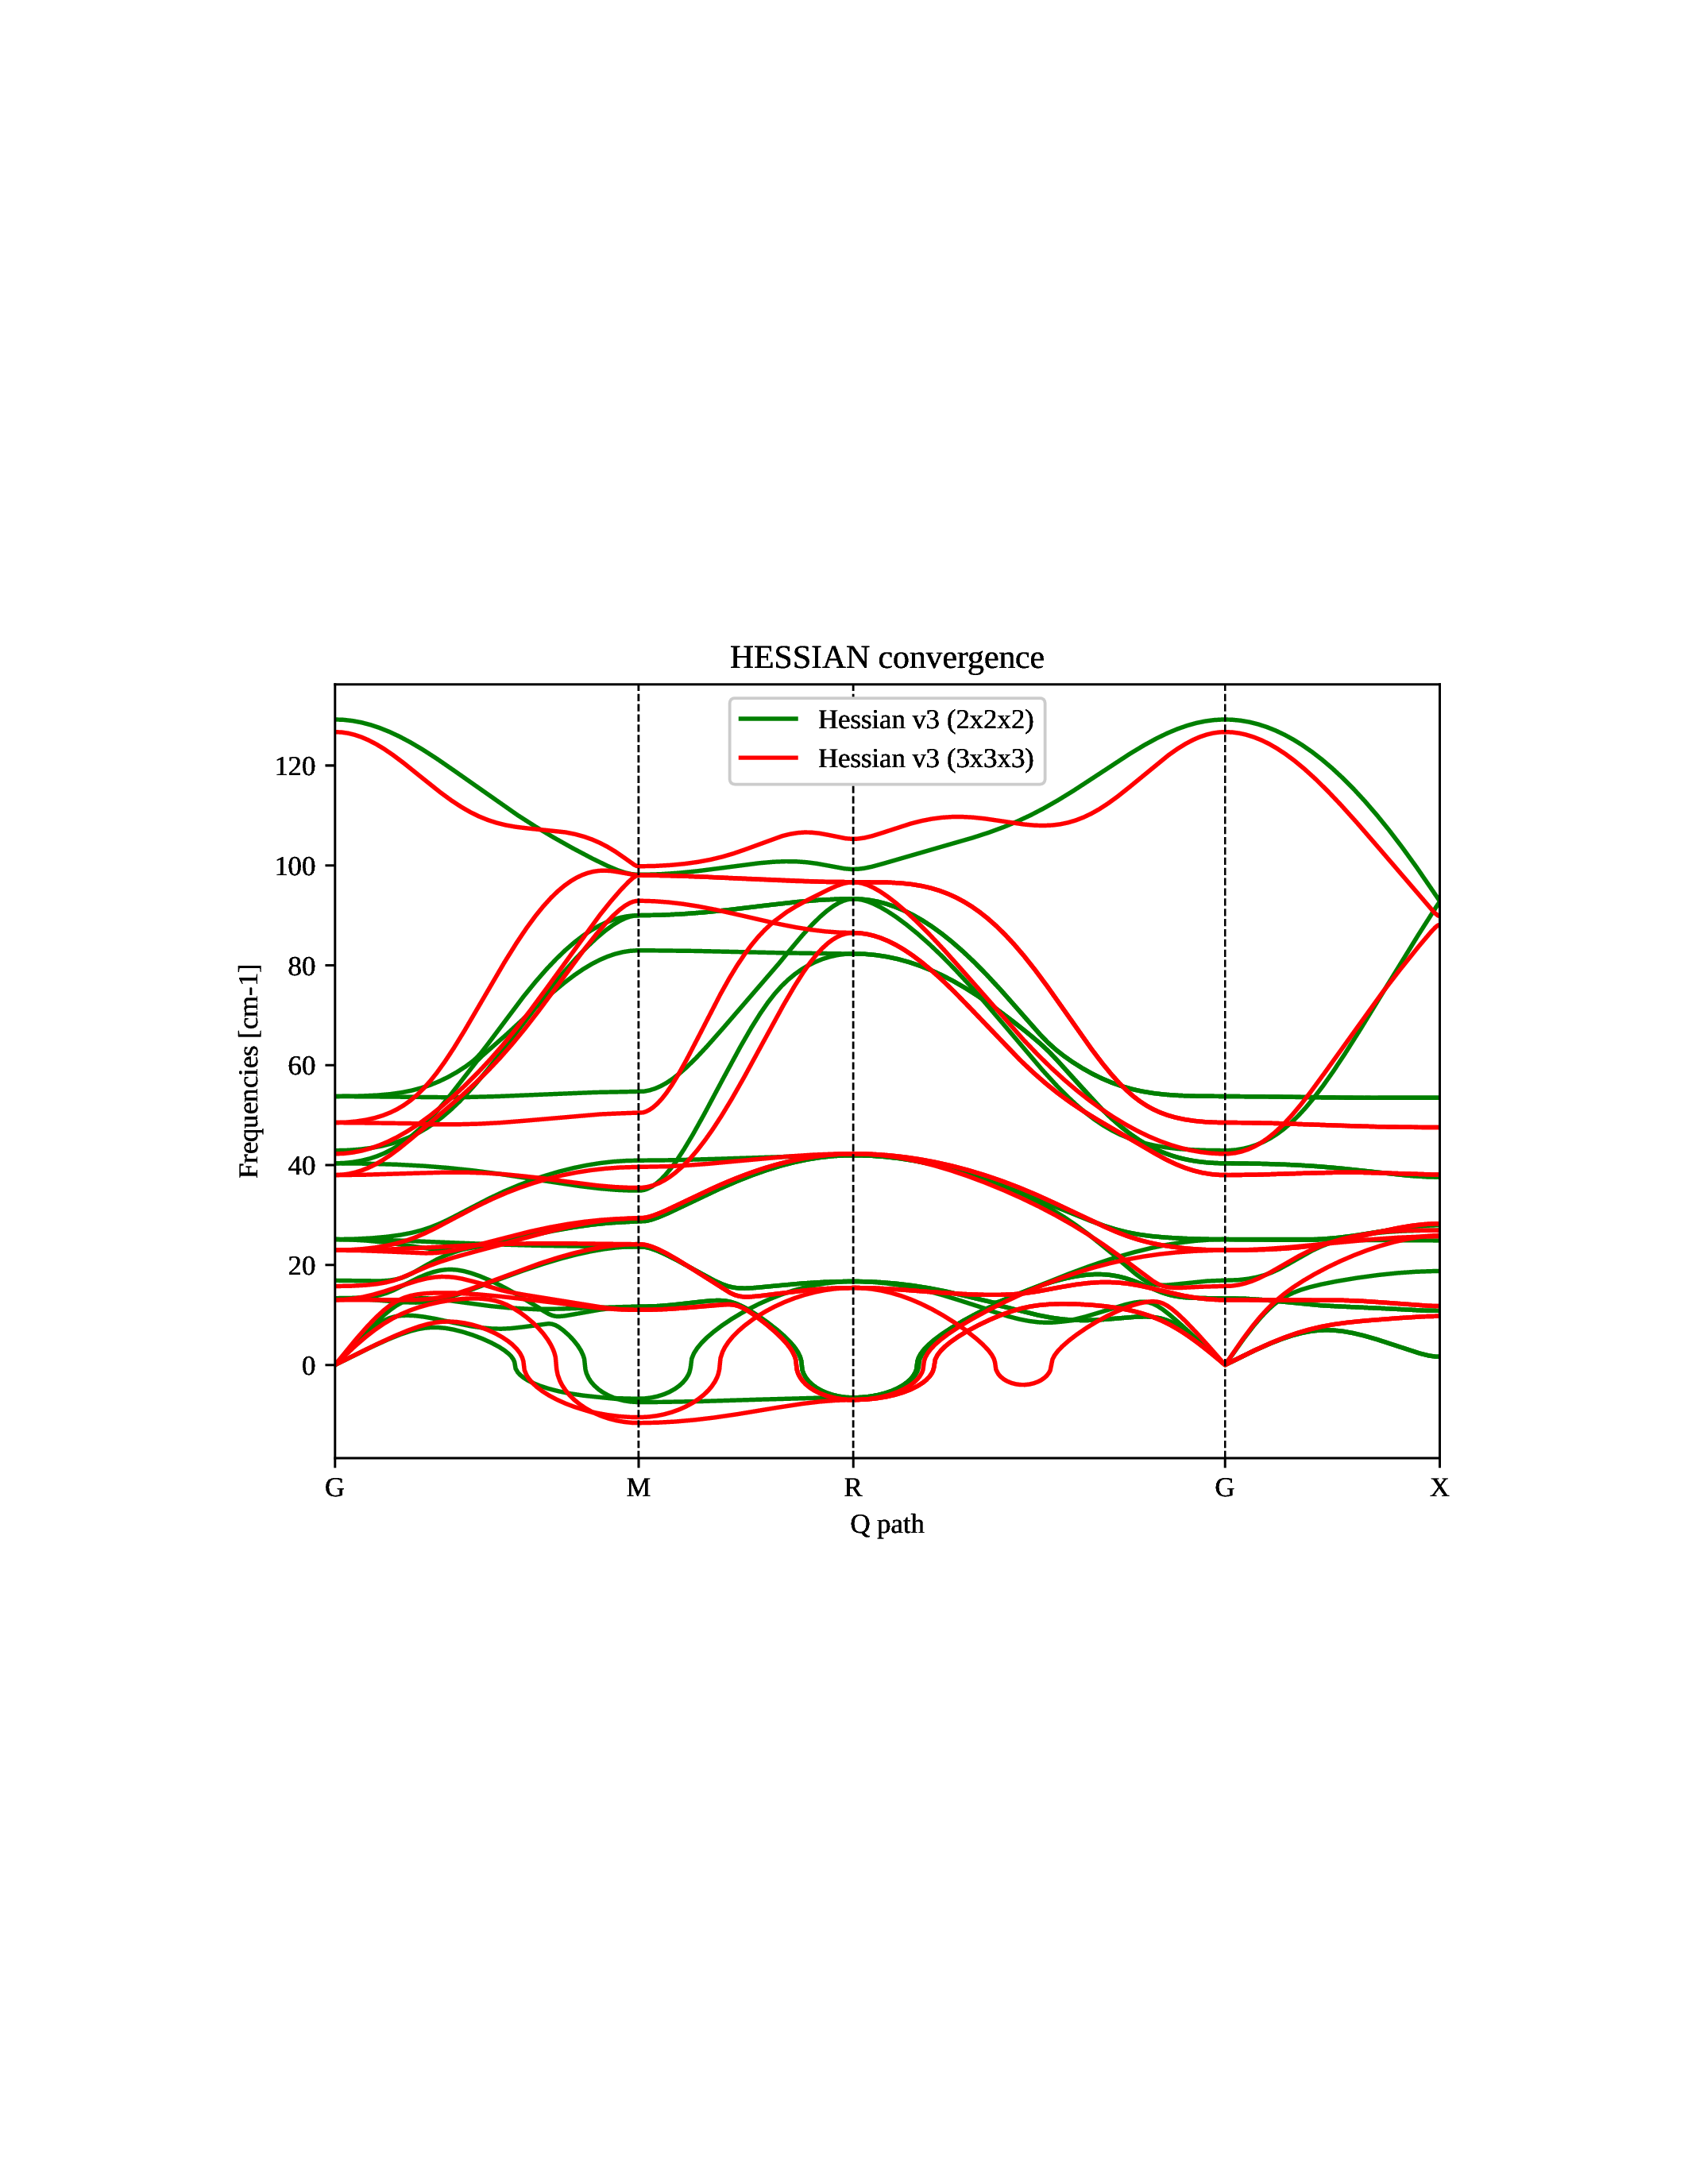}
	\caption{Convergence of the free energy hessian in the bubble approximation (v3) between the 2x2x2 and 3x3x3 supercell at \SI{300}{\kelvin}.\label{fig:bubble:conv}.}
\end{figure}

As can be seen, the $M-R$ path is almost overlapped, with a more pronounced instability at the $M$ mode. This difference comparable with the Fourier interpolation error. 
Another interesting point is an instability occurring between $R-\Gamma$ path, absent in the 2x2x2. 
This path is strongly affected by interpolation error of the 2x2x2, thus the new supercell is required.

From these data it seems that the calculation in the 2x2x2 has already a quite good convergence in the $R-M$, which is the dominant one for the stability.
However, the presence of the small instability between $R-\Gamma$ in the 3x3x3 is not converged in the 2x2x2, and requires the simulation of the full hessian in a bigger mesh to be checked. (\textbf{TODO: check if it a point commensurate with the 3x3x3, then we can run the Lanczos to get that frequency with the full hessian.})

.
