# Supplementary material for: First-principles thermodynamics of CsSnI3
Source: arXiv:2301.10071 source file (2023-01-24)
Supplement: Supplementary file 4 [file thermal_expansion.tex]

\section{Thermal expansion}

The \ch{CsSnI3} was reported to be one of the largest observed experimentally.
In particular, the orthorhombic phase at room temperature exhibits a volume thermal expansion of \SI{126e-6}{\per\kelvin}.\cite{Chung2012}.

Here, we report the thermal expansion computed for the two temperatures simulated at $T = \SI{300}{\kelvin}$ and $\SI{800}{\kelvin}$.

The overall volume thermal expansion coefficient is for the cubic phase is $\alpha = \SI{83e-6}{\per\kelvin}$, which confirms the experimental result of \ch{CsSnI3} as one of the largest volumetric expansion among solids (for comparison, \ch{Al} has $\alpha = \SI{75e-6}{\per\kelvin}$)

The volume expansion is reported in \figurename~\ref{fig:cubic:volume:expansion}.

\begin{figure}
	\includegraphics[width=\textwidth]{thermal_expansion_cubic.eps}
	\caption{Thermal expansion of cubic \ch{CsSnI3} obtained from SCHA simulations in the 2x2x2 supercell.}
	\label{fig:cubic:volume:expansion}
\end{figure}

The result is converged with the cell size, as the pressure at fixed volume for the starting calculation is \SI{-0.618\pm0.002}{\giga\pascal} in the 3x3x3 supercell and \SI{-0.633\pm0.003}{\giga\pascal} in the 2x2x2 supercell. Thus, the contribution of the cell size only affects the final volume of about \SI{0.3}{\angstrom^3} per unit cell and a resulting error on the $\alpha$ thermal expansion coefficient of about \SI{3}{\percent}.
